# Supplementary material for: Box Supervised Video Segmentation Proposal Network
Source: arXiv:2202.07025 source file (2022-02-16)
Supplement: Supplementary file 1 [file 08-Appendix.tex]

\chapter{Appendix}
\label{appndx}

\section{More Qualitative Studies}
In addition to the qualitative example presented in the main paper, we have created a video containing five positive and one negative example. Similar to Figure \ref{fig:example}, a sample video\footnote{https://drive.google.com/file/d/1fFMTctU8HyXMjbiXKRjCt1HOfosjdiQz/view?usp=sharing} contained the input frames, ground truth, various motion maps and predicted masks for better comparisons. One such example can be seen in Fig. \ref{fig:example}

\begin{figure}[!htp]
\centering
\includegraphics[width=\linewidth]{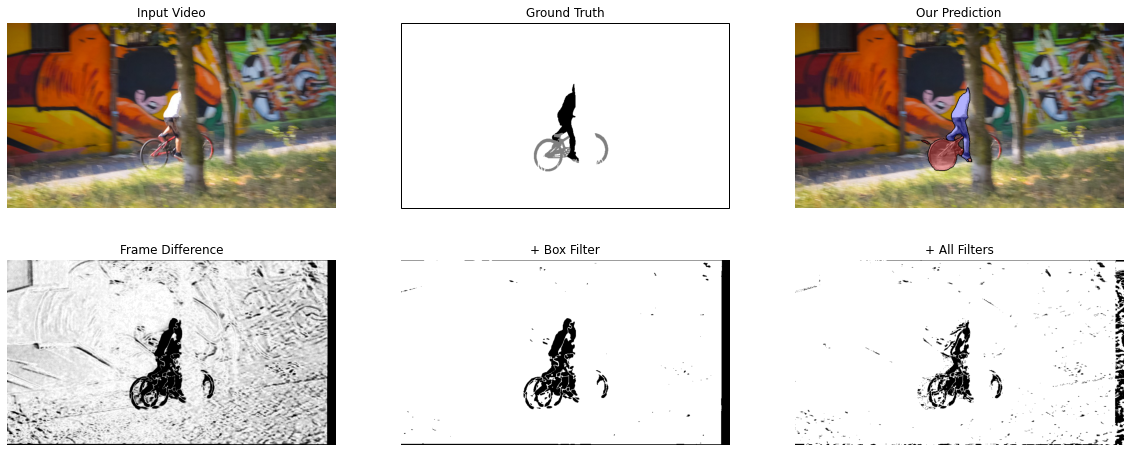}
\caption{\textbf{An example frame from the video sequence.} First column represents side-by-side portraying of input, ground truth and prediction. Moreover the second column shows proposed sequential improvement of motion map.}
\label{fig:example}
\end{figure}

In Fig. \ref{fig:c_v_m}, more example prediction is visualized where the advantage of incorporating motion on top of color is shown. The animal's color has similarities with the shell, and the color-only model could not differentiate between the two instances. Whereas, our approach could successfully discriminate between them. Hence the motion inclusion is advantageous in this case.

\begin{figure}[h]
    \centering
    \includegraphics[width=1\linewidth]{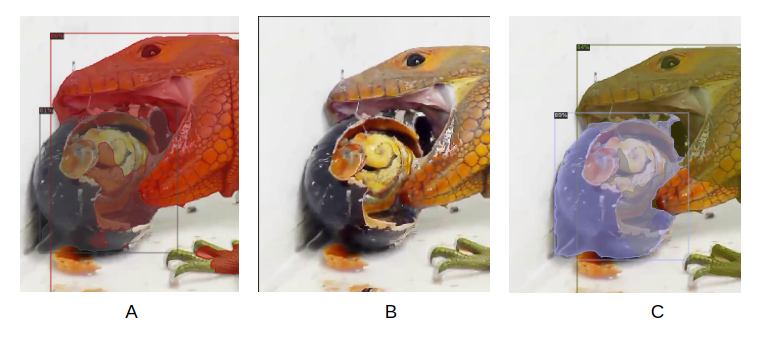}
    \caption{Comparison between baseline and MBVOS on YoutubeVOS dataset. The shell has similar color as the animal, hence only color similarity predicts part of the shell as the animal. With motion information, the animal can be differentiated from the shell with MBVOS.}
    \label{fig:c_v_m}
\end{figure}

\section{Further Hyper-Parameter Search}
Apart from the core ablation studies, more hyper-parameter tuning was performed. One important result in table \ref{tab:more_hpo} shows that taking motion as input into neural network does not improve the performance. We tried to inject motion in 5 different layers of ResNet-50 model, i.e., after the first conv layer, and subsequent blocks. The late fusion worked better than early fusion because the network could independently encode motion feature and then fuse at the later stages. But the approach could not achieve best result. So injecting motion inside the network is not necessary. Because we don't need to calculate motion and create different parameters to encode the motion during test time, the inference complexity is not increased by our approach.

\begin{table}[!htp]\centering
% \scriptsize
\begin{tabular}{c|c|c|c}\toprule
Filters &Supervision &Input &$\mathcal{J}\& \mathcal{F}($Mean$)$ \\\midrule\midrule
None &Color &Color &68.5(BoxInst $\dagger$) \\
None &Color $\cap$ Motion &Color &68.7 \\
FBF & Color $\cap$ Motion &Color & 68.9\\
3F & Color $\cap$ Motion &Color &69 \\
BF & Color $\cap$ Motion &Color &69.1 \\
3F + FBF &Color $\cap$ Motion &Color & 69.1 \\
3F + BF & Color $\cap$ Motion &Color &  69.2 \\
% 3F + BF + FBF & Color $\cap$ Motion & Color &70.5\\
\textbf{3F + BF + FBF} & \textbf{Color $\cap$ Motion} & \textbf{Color} &\textbf{70.5} \\
3F + BF + FBF  &Color $\cap$ Motion &Color + Motion & 69 \\
3F + BF + FBF  &Color $\cup$ Motion &Color & 68.6\\
3F + BF + FBF  & Motion &Color &66.3 \\
\bottomrule
\end{tabular}
    \begin{tablenotes}
        \smaller
        \item 
        \begin{center}
            3F: 3-Frame Difference, BF: Box Filter, FBF: Forward-Backward Filter
        \end{center}
    \end{tablenotes}
\caption{\centering Ablation Study for Motion on DAVIS dataset. $\dagger$ denotes adoption of the framework in video domain.}
\label{tab:more_hpo}
\end{table}

\pagebreak

% Set based Loss example: First we cluster pixels according to motion and consider only top 3 and bottom 3 motion groups. Then we cluster each of the 6 groups into 3 clusters based on color. In total we will have 18 groups/ sets. For each set we will force the network to predict the same label where we don’t care about the exact label.

\section{Visualization: Motion Calculation Pipeline}
Fig. \ref{fig:set_loss} shows all the intermediate steps' output of the proposed motion calculation pipeline. Before executing the motion compensation, the frames are transformed into gray images and a gaussian filter is applied to incur the blur effect. 

\begin{figure}[!htp]
\centering
\includegraphics[width=\linewidth]{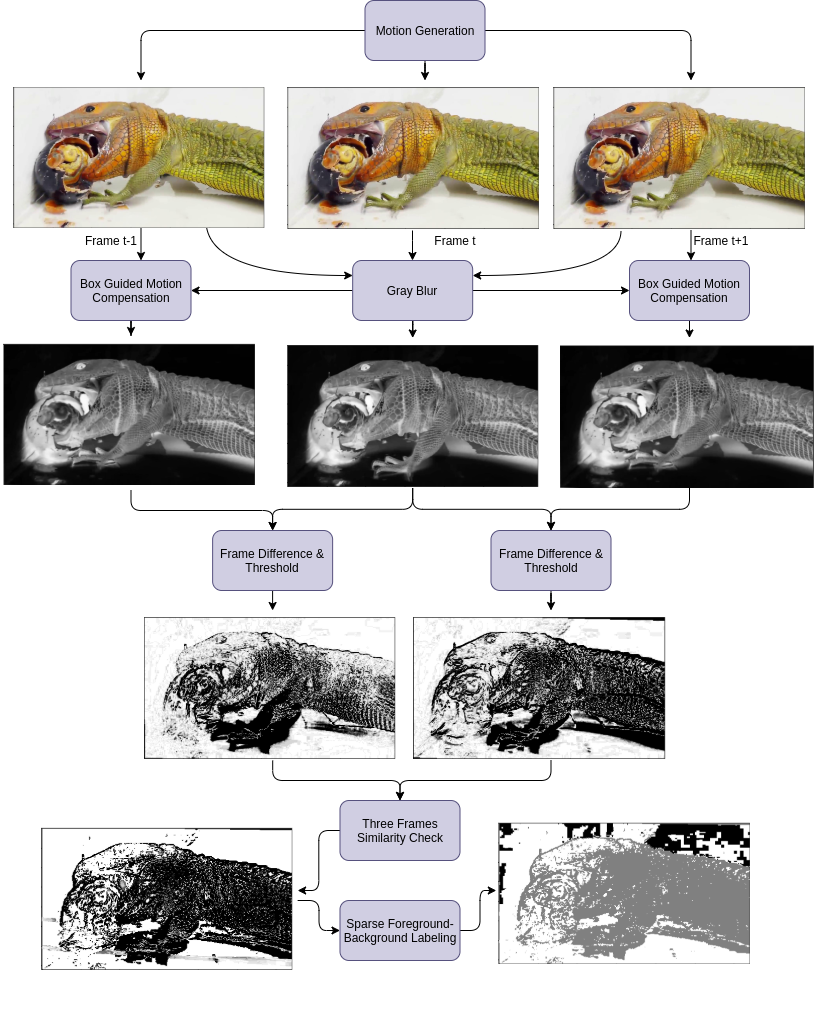}
\caption{Visualization of end to end motion calculation pipeline. The images are transformed into gray-scale ones before motion compensation initiates. }
\label{fig:set_loss}
\end{figure}
